# Supplementary material for: Enhanced Intrusion Detection in IIoT Networks: A Lightweight Approach with Autoencoder-Based Feature Learning
Source: arXiv:2501.15266 source file (2025-01-25)
Supplement: Supplementary file 1 [file appendice.tex]

\section{Appendices}\label{sec:Appendices}

\end{document}
